# Supplementary material for: Mechanisms for Global Differential Privacy under Bayesian Data Synthesis
Source: arXiv:2205.05003 source file (2023-08-03)
Supplement: Supplementary file 1 [file supp.pdf]

0.4pt=0pt

---

## **Mechanisms for Global Differential Privacy under Bayesian Data Synthesis**

*Vassar College, RTI International and U.S. Bureau of Labor Statistics*

### **Supplementary Material**

This Supplementary Material document contains: 1) Stan script for the censoring method for the beta synthesizer used in Section 4, 2) additional utility comparison results from Section 4.3, and 3) privacy and additional utility comparison results from Section 4.4.

## S1 Stan script for the censoring method for the beta synthesizer used in Section 4

Below we include the Stan script for our censoring method for the beta synthesizer used in our simulation study in Section 4. Note that the value  $M$  in the script is set as  $M = \epsilon/2$ .

```
functions{

  real betawt_lpdf(vector outcome, real beta1, real beta2, vector alpha, int n, real M)
  {
    real check_term;
    real update_term;
    check_term = 0.0;
    for( i in 1:n )
    {
      update_term = alpha[i] * beta_lpdf(outcome[i] | beta1, beta2);
      check_term = check_term + fmax(fmin(update_term, M), -M);
    }
    return check_term;
  }

  real betawt_i_lpdf(real outcome_i, real beta1, real beta2, real alpha_i, real M){
    real check_term;
    real update_term;
    update_term = alpha_i * beta_lpdf(outcome_i | beta1, beta2);
    check_term = fmax(fmin(update_term, M), -M);
    return check_term;
  }

  real betawt_i_noM_lpdf(real outcome_i, real beta1, real beta2, real alpha_i){
    real check_term;
    check_term = alpha_i * beta_lpdf(outcome_i | beta1, beta2);
    return check_term;
  }

} /* end function{} block */
```

```

data {
  int<lower=1> n; // number of observations
  vector[n] outcome; // Response variable
  vector<lower=0>[n] alpha; // observation-indexed (privacy) weights
  real<lower=0> M; //censoring threshold
}

parameters{
  real<lower=0,upper=1> phi;
  real<lower=0.1> lambda;
}

transformed parameters{
  real<lower=0> beta1 = lambda * phi;
  real<lower=0> beta2 = lambda * (1 - phi);
}

model{
  phi ~ beta(1, 1); // uniform on phi, could drop
  lambda ~ pareto(0.1, 1.5);

  target += betawt_lpdf(outcome | beta1, beta2, alpha, n, M);
} /* end model{} block */

generated quantities{
  vector[n] log_lik;
  vector[n] log_lik_noM;

  for (i in 1:n) {
    log_lik[i] = betawt_i_lpdf(outcome[i] | beta1, beta2, alpha[i], M);
    log_lik_noM[i] = betawt_i_noM_lpdf(outcome[i] | beta1, beta2, alpha[i]);
  }
}

```

## S2 Additional utility comparison results from Section 4.3

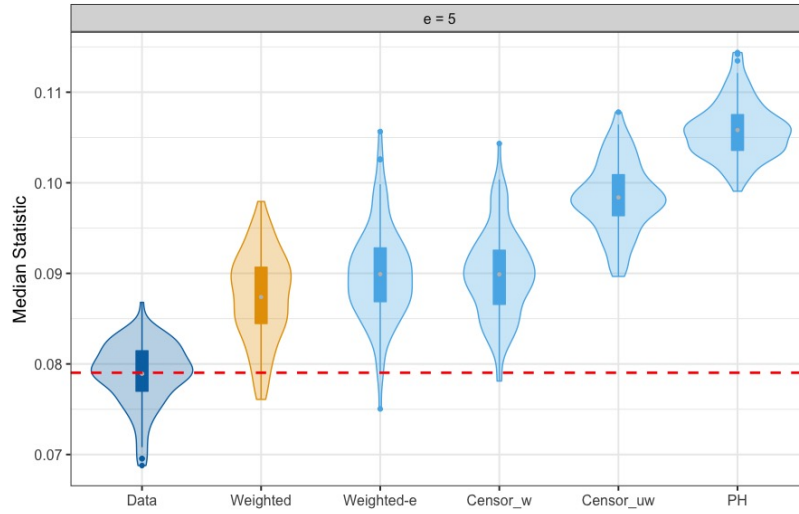

Figure 1: Violin plots of median over  $R = 100$  replicates for the Weighted, the Weighted-e, the Censor\_w, the Censor\_uw, and the PH, at  $\epsilon = 5$ . A dashed horizontal line at the analytical median from Beta(0.5, 3) is included.

## S2. ADDITIONAL UTILITY COMPARISON RESULTS FROM SECTION 4.3

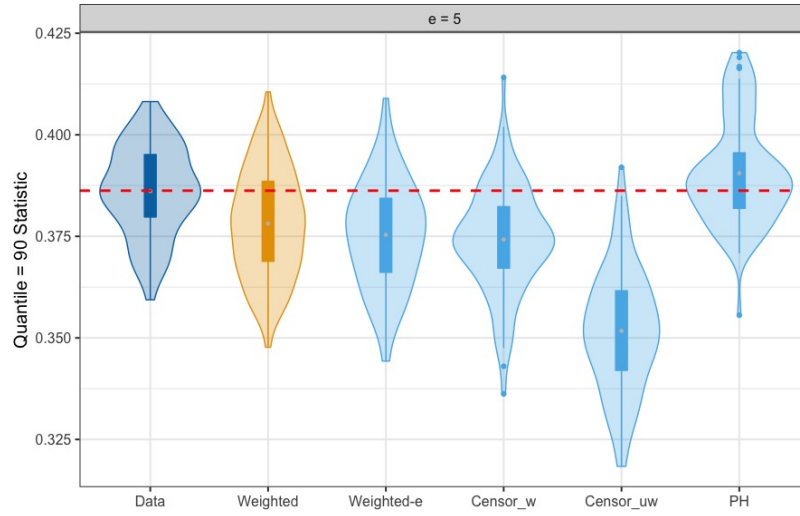

Figure 2: Violin plots of the 90th quantile over  $R = 100$  replicates for the Weighted, the Weighted-e, the Censor\_w, the Censor\_uw, and the PH, at  $\epsilon = 5$ . A dashed horizontal line at the analytical 90th quantile from Beta(0.5, 3) is included.

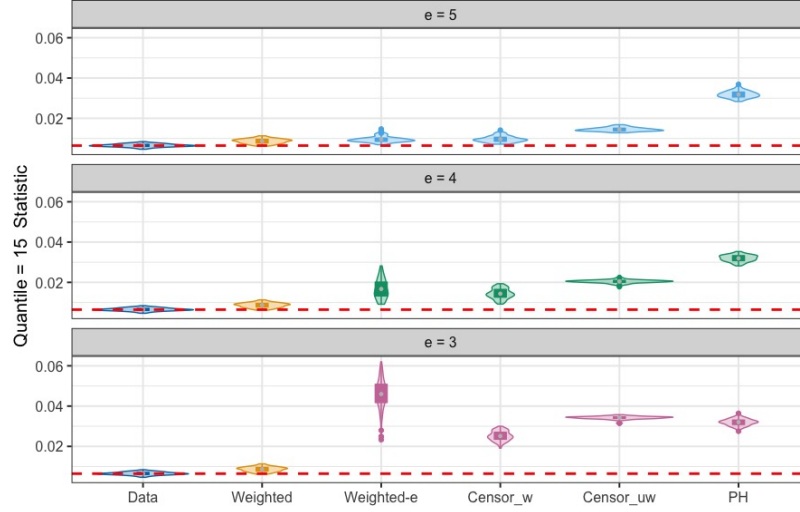

Figure 3: Violin plots of the 15th quantile over  $R = 100$  replicates, for the Weighted, the Weighted-e, the Censor\_w, the Censor\_uw, and the PH, with  $\epsilon$  values of  $\{5, 4, 3\}$ . A dashed horizontal line at the analytical 15h quantile from  $\text{Beta}(0.5, 3)$  is included in each panel.

## S2. ADDITIONAL UTILITY COMPARISON RESULTS FROM SECTION 4.3

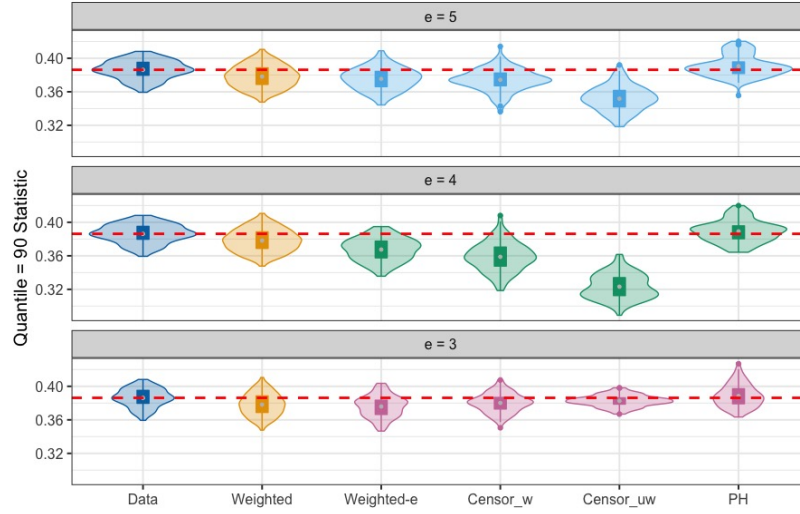

Figure 4: Violin plots of the 90th quantile over  $R = 100$  replicates, for the Weighted, the Weighted-e, the Censor\_w, the Censor\_uw, and the PH, with  $\epsilon$  values of  $\{5, 4, 3\}$ . A dashed horizontal line at the analytical 90th quantile from  $\text{Beta}(0.5, 3)$  is included in each panel.

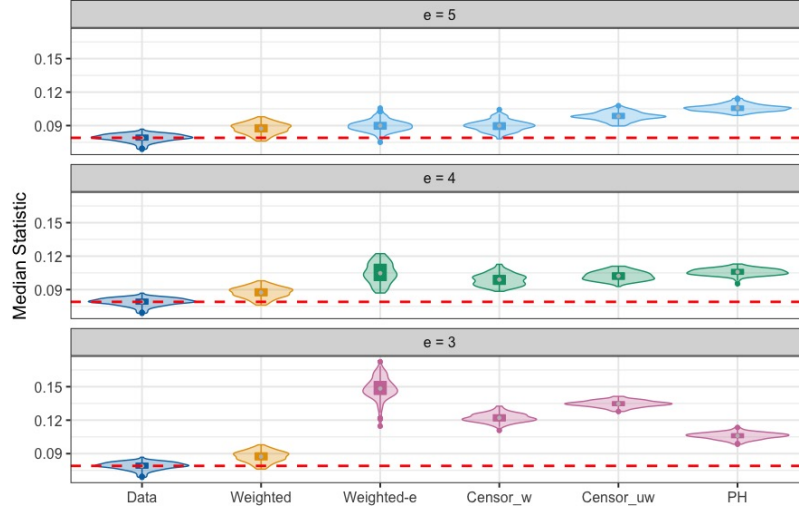

Figure 5: Violin plots of the median over  $R = 100$  replicates, for the Weighted, the Weighted-e, the Censor\_w, the Censor\_uw, and the PH, with  $\epsilon$  values of  $\{5, 4, 3\}$ . A dashed horizontal line at the analytical median from  $\text{Beta}(0.5, 3)$  is included in each panel.

### S3 Privacy and additional utility comparison results from Section 4.4

|                            |            | Min | Q1  | Median | Mean | Q3  | Max | sd     |
|----------------------------|------------|-----|-----|--------|------|-----|-----|--------|
| $\epsilon = 4$             | Weighted-e | 0   | 130 | 219    | 195  | 272 | 364 | 103.48 |
|                            | Censor_w   | 0   | 404 | 425    | 408  | 440 | 549 | 92.56  |
| $\epsilon = 4$ (downscale) | Weighted-e | 0   | 0   | 93     | 91   | 165 | 269 | 86.49  |
|                            | Censor_w   | 0   | 0   | 0      | 144  | 328 | 413 | 165.66 |

Table 1: Summaries of the number of records (out of  $n = 2000$ ) receiving truncated weight at  $\alpha_i = 0$  in Weighted-e and censored likelihood at  $\epsilon/2$  in Censor\_w. The number of Monte Carlo simulations is  $R = 100$ .

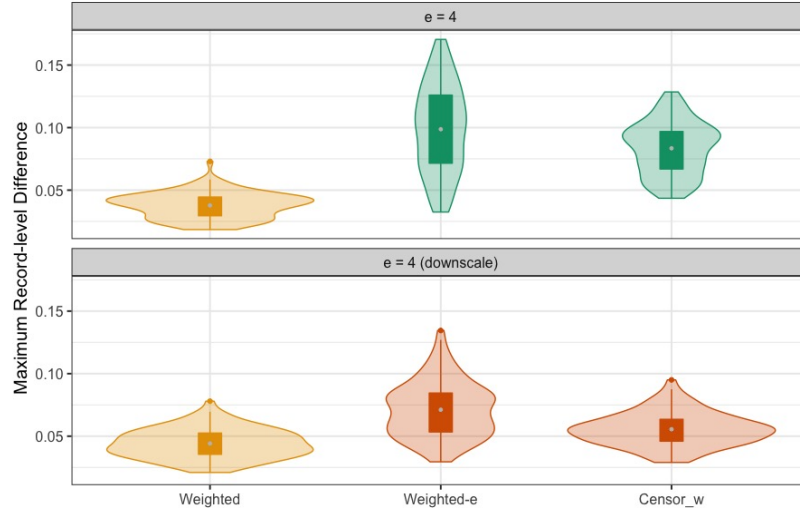

Figure 6: Violin plots of ECDF utility - maximum record-level difference over  $R = 100$  replicates, for the Weighted, the Weighted-e, and the Censor\_w at  $\epsilon = 4$ , without downscaling (top) and with downscaling (bottom).

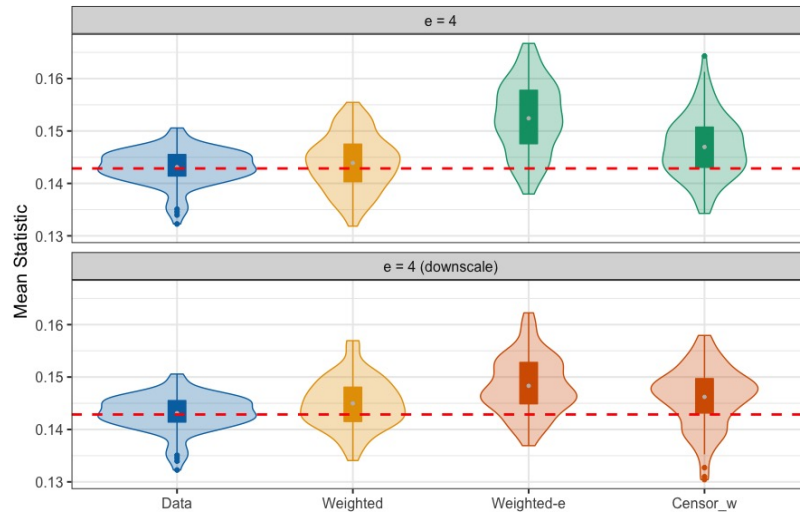

Figure 7: Violin plots of mean over  $R = 100$  replicates for the Weighted, the Weighted-e, and the Censor\_w at  $\epsilon = 4$ , without (top) and with (bottom) downscaling. A dashed horizontal line at the analytical mean from  $\text{Beta}(0.5, 3)$  is included in each panel.

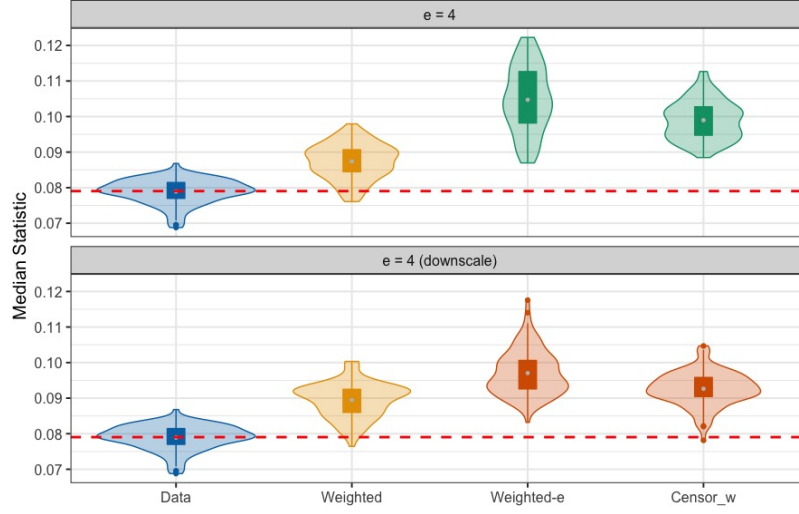

Figure 8: Violin plots of median over  $R = 100$  replicates for the Weighted, the Weighted-e, the Censor\_w, and the Censor\_uw at  $\epsilon = 4$ , without downscaling (top) and with downscaling (bottom). A dashed horizontal line at the analytical median from Beta(0.5, 3) is included in each panel.

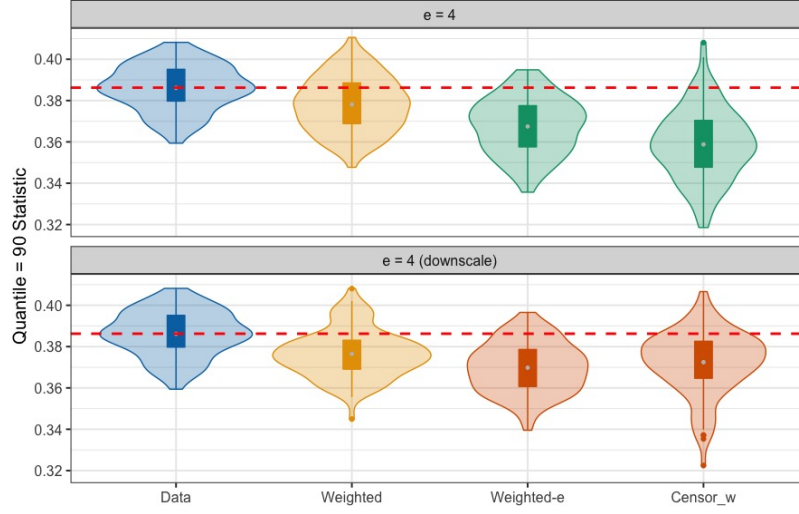

Figure 9: Violin plots of the 90th quantile over  $R = 100$  replicates for the Weighted, the Weighted-e, and the Censor\_w at  $\epsilon = 4$ , without downscaling (top) and with downscaling (bottom). A dashed horizontal line at the analytical 90th quantile from Beta(0.5, 3) is included in each panel.
